# Supplementary material for: Manipulation with Shared Grasping
Source: arXiv:2006.02996 source file (2020-06-04)
Supplement: Supplementary file 1 [file APPENDIX.tex]

% !TEX root = ../RSS20PartialGrasp.tex

\section*{APPENDIX}

\subsection{Stability Margin for Cone Intersection} % (fold)
\label{sub:stability_margin_for_cone_intersection}

% subsection stability_margin_for_cone_intersection (end)
